# Supplementary material for: MPRNet: Multi-Path Residual Network for Lightweight Image Super Resolution
Source: arXiv:2011.04566 source file (2020-11-09)
Supplement: Supplementary file 1 [file params.tex]

\begin{table*}[]
\begin{adjustbox}{width=1\textwidth}
\setlength\arrayrulewidth{1.0pt}
\begin{tabular}{|c|c|c|c|c|c|c|c|c|c|c|c|c|}
\hline

 & Method & \begin{tabular}[c]{@{}c@{}}\textbf{LapSRN}{\cite{lai2017deep}}\\ \hline Params-MAC\end{tabular} & \begin{tabular}[c]{@{}c@{}}\textbf{VDSR}{\cite{kim2016accurate}}\\ \hline Params-MAC\end{tabular} & \begin{tabular}[c]{@{}c@{}}\textbf{MemNet}{\cite{tai2017memnet}} \\ \hline Params-MAC\end{tabular} & \begin{tabular}[c]{@{}c@{}}\textbf{CARN}{\cite{ahn2018fast}}\\ \hline Params-MAC\end{tabular} & \begin{tabular}[c]{@{}c@{}}\textbf{FALSR-A}{\cite{chu2019fast}}\\ \hline Params-MAC\end{tabular} & \begin{tabular}[c]{@{}c@{}} \textbf{SRMDNF}{\cite{tong2017image}}\\ \hline Params-MAC\end{tabular} & \begin{tabular}[c]{@{}c@{}} \textbf{SRDenseNet}{\cite{zhang2018learning}}\\ \hline Params-MAC\end{tabular} & \begin{tabular}[c]{@{}c@{}}\textbf{OISR-LF-s}{\cite{he2019ode}}\\ \hline Params-MAC\end{tabular} & \begin{tabular}[c]{@{}c@{}}\textbf{MSRN}{\cite{li2018multi}}\\ \hline Params-MAC\end{tabular} &\begin{tabular}[c]{@{}c@{}}\textbf{RDN}{\cite{zhang2018residual}}\\ \hline Params-MAC\end{tabular} &
 \begin{tabular}[c]{@{}c@{}}\textbf{MPRNet[Ours]}\\ \hline Params-MAC\end{tabular} \\ \hline \hline
Scale & \begin{tabular}[c]{@{}c@{}}$\times2$\\ $\times3$\\ $\times4$\end{tabular} & \begin{tabular}[c]{@{}c@{}}813K-29G\\ -----\\ 813K-149.4G\end{tabular} & \begin{tabular}[c]{@{}c@{}}665K-612.6G\\ 665K-612.6G\\ 665K-612.6G\end{tabular} & \begin{tabular}[c]{@{}c@{}}677K-2662.4G\\ 667K-2662.4G\\ 667K-2662.4G\end{tabular} & \begin{tabular}[c]{@{}c@{}}1592K-222.8G\\ 1592K-118.8G\\ 1592K-90.9G\end{tabular} & \begin{tabular}[c]{@{}c@{}}1021K-234.7G\\ -----\\ -----\end{tabular} & \begin{tabular}[c]{@{}c@{}}1513K-347.7G\\ 1530K-156.3G\\ 1555K-89.3G\end{tabular} & \begin{tabular}[c]{@{}c@{}}-----\\ -----\\ 2015K-389.9G\end{tabular} & \begin{tabular}[c]{@{}c@{}}1370K-316.2G\\ 1550K-160.1G\\ 1552K-114.2G\end{tabular} & \begin{tabular}[c]{@{}c@{}}5930K-1365.8G\\ 6008K-621.2G\\ 6033K-365.1G\end{tabular} &
\begin{tabular}[c]{@{}c@{}}22120K-5096.2G\\ 22310K-2281.2G\\ 2227K-1309.2G\end{tabular} &
\begin{tabular}[c]{@{}c@{}}\textbf{461K-106.2G}\\ \textbf{509.8K-66.1G}\\ \textbf{509.8K-29G}\end{tabular} \\ \hline
\end{tabular}
\end{adjustbox}
\caption{Comparisons on the number of network parameters and MAC operations for all scale factors $[\times2, \times3, \times4]$ in detail (PSNR and SSIM are provided in the submitted manuscript).}
\label{tab:subparam}
\end{table*}
